# Supplementary material for: Sample complexity bounds for categorical Markov random fields via Discrete Diffusions
Source: arXiv:2610.02128 source file (2026-10-01)
Supplement: Supplementary file 1 [file additional.tex]

\multicolumn{5}{l}{\textit{Smaller Potts chain}} \\ \midrule
Score risk & $0.01013\,\pm\,0.00021$ & $\mathbf{0.00508\,\pm\,0.00018}$ & $0.01384\,\pm\,0.00096$ & $0.01009\,\pm\,0.00020$ \\
Centered DSE & $-0.0621\,\pm\,0.0008$ & $\mathbf{-0.0669\,\pm\,0.0013}$ & $-0.0580\,\pm\,0.0012$ & $-0.0619\,\pm\,0.0011$ \\
DSE obs. SD & $0.0476\,\pm\,0.0014$ & $0.0645\,\pm\,0.0022$ & $0.0589\,\pm\,0.0019$ & $0.0610\,\pm\,0.0022$ \\
Score MSE & $0.2329\,\pm\,0.0102$ & $\mathbf{0.1243\,\pm\,0.0079}$ & $0.2182\,\pm\,0.0122$ & $0.1801\,\pm\,0.0090$ \\
Log-score RMSE & $0.1897\,\pm\,0.0015$ & $\mathbf{0.1519\,\pm\,0.0024}$ & $0.2429\,\pm\,0.0077$ & $0.2053\,\pm\,0.0034$ \\
Mean site TV & $\mathbf{0.0266\,\pm\,0.0017}$ & $0.0382\,\pm\,0.0050$ & $0.0402\,\pm\,0.0041$ & $0.0311\,\pm\,0.0030$ \\
Mean edge TV & $0.1380\,\pm\,0.0036$ & $\mathbf{0.0742\,\pm\,0.0036}$ & $0.1267\,\pm\,0.0089$ & $0.0995\,\pm\,0.0052$ \\
Maximum edge TV & $0.1788\,\pm\,0.0057$ & $\mathbf{0.0984\,\pm\,0.0031}$ & $0.1992\,\pm\,0.0145$ & $0.1316\,\pm\,0.0065$ \\
Agreement RMSE & $0.1405\,\pm\,0.0035$ & $\mathbf{0.0552\,\pm\,0.0050}$ & $0.1266\,\pm\,0.0095$ & $0.0953\,\pm\,0.0068$ \\
Order $W_1$ & $0.1686\,\pm\,0.0035$ & $\mathbf{0.0538\,\pm\,0.0039}$ & $0.0806\,\pm\,0.0084$ & $0.0666\,\pm\,0.0055$ \\
Joint TV & $0.3368\,\pm\,0.0027$ & $\mathbf{0.1337\,\pm\,0.0064}$ & $0.2951\,\pm\,0.0157$ & $0.2178\,\pm\,0.0115$ \\
Forward KL & $0.3450\,\pm\,0.0060$ & $\mathbf{0.0670\,\pm\,0.0058}$ & $0.2805\,\pm\,0.0287$ & $0.1562\,\pm\,0.0123$ \\
Joint JS & $0.0831\,\pm\,0.0014$ & $\mathbf{0.0181\,\pm\,0.0016}$ & $0.0774\,\pm\,0.0074$ & $0.0434\,\pm\,0.0034$ \\
Joint $H^2$ & $0.0861\,\pm\,0.0015$ & $\mathbf{0.0186\,\pm\,0.0017}$ & $0.0836\,\pm\,0.0082$ & $0.0456\,\pm\,0.0037$ \\
\addlinespace[3pt]
\multicolumn{5}{l}{\textit{Smaller Ising ladder}} \\ \midrule
Score risk & $\mathbf{0.00166\,\pm\,0.00007}$ & $0.00360\,\pm\,0.00013$ & $0.00454\,\pm\,0.00019$ & $0.00327\,\pm\,0.00017$ \\
Centered DSE & $\mathbf{-0.0409\,\pm\,0.0005}$ & $-0.0390\,\pm\,0.0005$ & $-0.0379\,\pm\,0.0005$ & $-0.0393\,\pm\,0.0006$ \\
DSE obs. SD & $0.0438\,\pm\,0.0025$ & $0.0423\,\pm\,0.0019$ & $0.0400\,\pm\,0.0018$ & $0.0443\,\pm\,0.0021$ \\
Score MSE & $\mathbf{0.1276\,\pm\,0.0129}$ & $0.1951\,\pm\,0.0197$ & $0.2142\,\pm\,0.0194$ & $0.1858\,\pm\,0.0200$ \\
Log-score RMSE & $\mathbf{0.0890\,\pm\,0.0008}$ & $0.1606\,\pm\,0.0020$ & $0.1839\,\pm\,0.0036$ & $0.1533\,\pm\,0.0026$ \\
Mean site TV & $0.0202\,\pm\,0.0024$ & $0.0269\,\pm\,0.0030$ & $0.0236\,\pm\,0.0028$ & $\mathbf{0.0196\,\pm\,0.0024}$ \\
Mean edge TV & $0.0372\,\pm\,0.0027$ & $0.0462\,\pm\,0.0028$ & $0.0480\,\pm\,0.0034$ & $\mathbf{0.0354\,\pm\,0.0019}$ \\
Maximum edge TV & $0.0611\,\pm\,0.0026$ & $0.0703\,\pm\,0.0037$ & $0.0772\,\pm\,0.0053$ & $\mathbf{0.0565\,\pm\,0.0024}$ \\
Agreement RMSE & $0.0305\,\pm\,0.0012$ & $0.0339\,\pm\,0.0016$ & $0.0420\,\pm\,0.0023$ & $\mathbf{0.0258\,\pm\,0.0018}$ \\
Order $W_1$ & $0.0353\,\pm\,0.0038$ & $0.0284\,\pm\,0.0042$ & $0.0344\,\pm\,0.0046$ & $\mathbf{0.0198\,\pm\,0.0037}$ \\
Joint TV & $0.0983\,\pm\,0.0019$ & $0.1154\,\pm\,0.0042$ & $0.1408\,\pm\,0.0056$ & $\mathbf{0.0815\,\pm\,0.0053}$ \\
Forward KL & $0.0441\,\pm\,0.0015$ & $0.0645\,\pm\,0.0039$ & $0.0952\,\pm\,0.0053$ & $\mathbf{0.0425\,\pm\,0.0050}$ \\
Joint JS & $\mathbf{0.0122\,\pm\,0.0004}$ & $0.0184\,\pm\,0.0012$ & $0.0280\,\pm\,0.0016$ & $0.0123\,\pm\,0.0015$ \\
Joint $H^2$ & $\mathbf{0.0125\,\pm\,0.0004}$ & $0.0192\,\pm\,0.0012$ & $0.0299\,\pm\,0.0018$ & $0.0130\,\pm\,0.0016$ \\
\addlinespace[3pt]
\multicolumn{5}{l}{\textit{Smaller Categorical tree}} \\ \midrule
Score risk & $\mathbf{0.00138\,\pm\,0.00004}$ & $0.00493\,\pm\,0.00015$ & $0.00551\,\pm\,0.00015$ & $0.00381\,\pm\,0.00009$ \\
Centered DSE & $\mathbf{-0.0228\,\pm\,0.0008}$ & $-0.0190\,\pm\,0.0008$ & $-0.0187\,\pm\,0.0008$ & $-0.0204\,\pm\,0.0007$ \\
DSE obs. SD & $0.0359\,\pm\,0.0011$ & $0.0350\,\pm\,0.0012$ & $0.0340\,\pm\,0.0011$ & $0.0360\,\pm\,0.0012$ \\
Score MSE & $\mathbf{0.0163\,\pm\,0.0010}$ & $0.0288\,\pm\,0.0012$ & $0.0320\,\pm\,0.0009$ & $0.0241\,\pm\,0.0010$ \\
Log-score RMSE & $\mathbf{0.0669\,\pm\,0.0006}$ & $0.1353\,\pm\,0.0023$ & $0.1420\,\pm\,0.0025$ & $0.1159\,\pm\,0.0015$ \\
Mean site TV & $\mathbf{0.0273\,\pm\,0.0024}$ & $0.0296\,\pm\,0.0026$ & $0.0280\,\pm\,0.0017$ & $0.0329\,\pm\,0.0024$ \\
Mean edge TV & $\mathbf{0.0613\,\pm\,0.0017}$ & $0.0905\,\pm\,0.0047$ & $0.0984\,\pm\,0.0033$ & $0.0761\,\pm\,0.0024$ \\
Maximum edge TV & $\mathbf{0.0850\,\pm\,0.0030}$ & $0.1378\,\pm\,0.0103$ & $0.1625\,\pm\,0.0074$ & $0.1016\,\pm\,0.0035$ \\
Agreement RMSE & $\mathbf{0.0272\,\pm\,0.0024}$ & $0.0582\,\pm\,0.0040$ & $0.0540\,\pm\,0.0024$ & $0.0357\,\pm\,0.0024$ \\
Order $W_1$ & $0.0104\,\pm\,0.0014$ & $\mathbf{0.0102\,\pm\,0.0021}$ & $0.0108\,\pm\,0.0024$ & $0.0113\,\pm\,0.0016$ \\
Joint TV & $\mathbf{0.1039\,\pm\,0.0014}$ & $0.1886\,\pm\,0.0051$ & $0.2149\,\pm\,0.0049$ & $0.1367\,\pm\,0.0037$ \\
Forward KL & $\mathbf{0.0373\,\pm\,0.0009}$ & $0.1183\,\pm\,0.0061$ & $0.1508\,\pm\,0.0064$ & $0.0615\,\pm\,0.0031$ \\
Joint JS & $\mathbf{0.0099\,\pm\,0.0003}$ & $0.0300\,\pm\,0.0015$ & $0.0388\,\pm\,0.0016$ & $0.0159\,\pm\,0.0008$ \\
Joint $H^2$ & $\mathbf{0.0100\,\pm\,0.0003}$ & $0.0306\,\pm\,0.0016$ & $0.0397\,\pm\,0.0017$ & $0.0161\,\pm\,0.0008$ \\
\addlinespace[3pt]
\multicolumn{5}{l}{\textit{Larger Potts chain}} \\ \midrule
Score risk & $0.01079\,\pm\,0.00011$ & $\mathbf{0.00671\,\pm\,0.00091}$ & $0.05286\,\pm\,0.00091$ & $0.05617\,\pm\,0.00042$ \\
Centered DSE & $-0.0679\,\pm\,0.0005$ & $\mathbf{-0.0721\,\pm\,0.0010}$ & $-0.0253\,\pm\,0.0008$ & $-0.0224\,\pm\,0.0006$ \\
DSE obs. SD & $0.0254\,\pm\,0.0004$ & $0.0320\,\pm\,0.0012$ & $0.0181\,\pm\,0.0005$ & $0.0150\,\pm\,0.0005$ \\
Score MSE & $0.2421\,\pm\,0.0033$ & $\mathbf{0.1491\,\pm\,0.0205}$ & $0.5144\,\pm\,0.0070$ & $0.5324\,\pm\,0.0061$ \\
Log-score RMSE & $0.1983\,\pm\,0.0012$ & $\mathbf{0.1491\,\pm\,0.0054}$ & $0.4518\,\pm\,0.0066$ & $0.4609\,\pm\,0.0047$ \\
Mean site TV & $\mathbf{0.0258\,\pm\,0.0010}$ & $0.0359\,\pm\,0.0025$ & $0.0358\,\pm\,0.0010$ & $0.0317\,\pm\,0.0007$ \\
Mean edge TV & $0.1356\,\pm\,0.0012$ & $\mathbf{0.1017\,\pm\,0.0119}$ & $0.3652\,\pm\,0.0037$ & $0.3817\,\pm\,0.0034$ \\
Maximum edge TV & $0.1891\,\pm\,0.0029$ & $\mathbf{0.1539\,\pm\,0.0127}$ & $0.5012\,\pm\,0.0062$ & $0.5173\,\pm\,0.0052$ \\
Agreement RMSE & $0.1380\,\pm\,0.0014$ & $\mathbf{0.0955\,\pm\,0.0139}$ & $0.3765\,\pm\,0.0039$ & $0.3894\,\pm\,0.0030$ \\
Order $W_1$ & $0.0991\,\pm\,0.0019$ & $\mathbf{0.0500\,\pm\,0.0056}$ & $0.1387\,\pm\,0.0036$ & $0.1529\,\pm\,0.0021$ \\
\addlinespace[3pt]
\multicolumn{5}{l}{\textit{Larger Ising ladder}} \\ \midrule
Score risk & $\mathbf{0.00138\,\pm\,0.00002}$ & $0.01007\,\pm\,0.00064$ & $0.01324\,\pm\,0.00052$ & $0.01947\,\pm\,0.00033$ \\
Centered DSE & $\mathbf{-0.0460\,\pm\,0.0006}$ & $-0.0372\,\pm\,0.0006$ & $-0.0343\,\pm\,0.0005$ & $-0.0278\,\pm\,0.0004$ \\
DSE obs. SD & $0.0251\,\pm\,0.0007$ & $0.0206\,\pm\,0.0006$ & $0.0191\,\pm\,0.0004$ & $0.0174\,\pm\,0.0006$ \\
Score MSE & $\mathbf{0.1148\,\pm\,0.0093}$ & $0.2907\,\pm\,0.0206$ & $0.3445\,\pm\,0.0194$ & $0.3988\,\pm\,0.0209$ \\
Log-score RMSE & $\mathbf{0.0790\,\pm\,0.0007}$ & $0.2276\,\pm\,0.0060$ & $0.2704\,\pm\,0.0059$ & $0.3296\,\pm\,0.0028$ \\
Mean site TV & $\mathbf{0.0185\,\pm\,0.0010}$ & $0.0365\,\pm\,0.0054$ & $0.0309\,\pm\,0.0019$ & $0.0239\,\pm\,0.0014$ \\
Mean edge TV & $\mathbf{0.0333\,\pm\,0.0011}$ & $0.1009\,\pm\,0.0073$ & $0.0951\,\pm\,0.0030$ & $0.1360\,\pm\,0.0034$ \\
Maximum edge TV & $\mathbf{0.0682\,\pm\,0.0034}$ & $0.2233\,\pm\,0.0183$ & $0.2403\,\pm\,0.0179$ & $0.3191\,\pm\,0.0055$ \\
Agreement RMSE & $\mathbf{0.0267\,\pm\,0.0008}$ & $0.1075\,\pm\,0.0095$ & $0.1022\,\pm\,0.0043$ & $0.1506\,\pm\,0.0029$ \\
Order $W_1$ & $0.0156\,\pm\,0.0018$ & $\mathbf{0.0131\,\pm\,0.0027}$ & $0.0265\,\pm\,0.0020$ & $0.0495\,\pm\,0.0022$ \\
\addlinespace[3pt]
\multicolumn{5}{l}{\textit{Larger Categorical tree}} \\ \midrule
Score risk & $\mathbf{0.00136\,\pm\,0.00003}$ & $0.01588\,\pm\,0.00024$ & $0.01526\,\pm\,0.00015$ & $0.01735\,\pm\,0.00011$ \\
Centered DSE & $\mathbf{-0.0249\,\pm\,0.0004}$ & $-0.0103\,\pm\,0.0003$ & $-0.0108\,\pm\,0.0003$ & $-0.0088\,\pm\,0.0003$ \\
DSE obs. SD & $0.0192\,\pm\,0.0003$ & $0.0131\,\pm\,0.0004$ & $0.0136\,\pm\,0.0003$ & $0.0118\,\pm\,0.0004$ \\
Score MSE & $\mathbf{0.0190\,\pm\,0.0032}$ & $0.0905\,\pm\,0.0058$ & $0.0865\,\pm\,0.0053$ & $0.0933\,\pm\,0.0055$ \\
Log-score RMSE & $\mathbf{0.0660\,\pm\,0.0008}$ & $0.2366\,\pm\,0.0017$ & $0.2322\,\pm\,0.0014$ & $0.2429\,\pm\,0.0011$ \\
Mean site TV & $\mathbf{0.0263\,\pm\,0.0005}$ & $0.0423\,\pm\,0.0018$ & $0.0319\,\pm\,0.0010$ & $0.0585\,\pm\,0.0020$ \\
Mean edge TV & $\mathbf{0.0599\,\pm\,0.0009}$ & $0.1669\,\pm\,0.0020$ & $0.1647\,\pm\,0.0014$ & $0.1795\,\pm\,0.0014$ \\
Maximum edge TV & $\mathbf{0.0981\,\pm\,0.0025}$ & $0.3193\,\pm\,0.0036$ & $0.3340\,\pm\,0.0033$ & $0.3371\,\pm\,0.0076$ \\
Agreement RMSE & $\mathbf{0.0268\,\pm\,0.0010}$ & $0.0880\,\pm\,0.0014$ & $0.0895\,\pm\,0.0017$ & $0.0984\,\pm\,0.0015$ \\
Order $W_1$ & $0.0046\,\pm\,0.0006$ & $0.0063\,\pm\,0.0008$ & $0.0045\,\pm\,0.0004$ & $\mathbf{0.0044\,\pm\,0.0005}$ \\
\addlinespace[3pt]
